# Supplementary material for: DiffSensei: Bridging Multi-Modal LLMs and Diffusion Models for Customized Manga Generation
Source: arXiv:2412.07589 source file (2025-03-13)
Supplement: Supplementary file 1 [file supplementary.tex]

% CVPR 2024 Paper Template; see https://github.com/cvpr-org/author-kit

\documentclass[10pt,twocolumn,letterpaper]{article}

%%%%%%%%% PAPER TYPE  - PLEASE UPDATE FOR FINAL VERSION
\usepackage[review]{cvpr}              % To produce the CAMERA-READY version
% \usepackage[review]{cvpr}      % To produce the REVIEW version
% \usepackage[pagenumbers]{cvpr} % To force page numbers, e.g. for an arXiv version

% Import additional packages in the preamble file, before hyperref
% \input{preamble}

% It is strongly recommended to use hyperref, especially for the review version.
% hyperref with option pagebackref eases the reviewers' job.
% Please disable hyperref *only* if you encounter grave issues, 
% e.g. with the file validation for the camera-ready version.
%
% If you comment hyperref and then uncomment it, you should delete *.aux before re-running LaTeX.
% (Or just hit 'q' on the first LaTeX run, let it finish, and you should be clear).
% Include other packages here, before hyperref.
\usepackage{graphicx}
\usepackage{amsmath}
\usepackage{amssymb}
\usepackage{amsfonts}
\usepackage{booktabs}
\usepackage{color}
\usepackage[table]{xcolor}
\usepackage{multirow}
\usepackage{subcaption}
\usepackage{caption}

 % xiangtai's comments

% For reference link
% \definecolor{linkcolor}{RGB}{255,0,0}
% \definecolor{urlcolor}{RGB}{255,105,180}
% \definecolor{citecolor}{RGB}{66,168,235}
% \usepackage[pagebackref,breaklinks,colorlinks]{hyperref}
% \hypersetup{colorlinks=true,linkcolor=linkcolor,urlcolor=urlcolor,citecolor=citecolor}

% For reference link
\usepackage[pagebackref,breaklinks=true,colorlinks,citecolor=blue,urlcolor=blue,linkcolor=blue,bookmarks=false]{hyperref}

% Support for easy cross-referencing
%%%%%%%%% PAPER ID  - PLEASE UPDATE
 % *** Enter the Paper ID here

%%%%%%%%% TITLE - PLEASE UPDATE
\title{DiffSensei: Bridging Multi-Modal LLMs and Diffusion Models \\ for Customized Manga Generation Supplementary}

%%%%%%%%% AUTHORS - PLEASE UPDATE
\author{
    Jianzong Wu$^{1,2}$\thanks{The work is done during the internship at Shanghai AI Laboratory. \textsuperscript{$\dagger$}: Project Lead and corresponding author. Email: xiangtai94@gmail.com} \quad Xiangtai Li$^{2}$ \textsuperscript{$\dagger$} \quad Yunhai Tong$^{1,3}$ \\
    {\normalsize $^1$ National Key Laboratory of General Artificial Intelligence, Peking University} \\
    {\normalsize  $^2$Shanghai AI Laboratory  \quad 
    $^3$ PKU-Wuhan Institute for Artificial Intelligence} \\
    {\normalsize Project Page: \url{TODO}}
}

\begin{document}
\maketitle
\appendix

\input{latex/7_appendix}

{
    \small
    \bibliographystyle{ieee_fullname}
    \bibliography{egbib}
}

\end{document}
